# Supplementary material for: Simulation of charged nanotubes self-assembly during evaporation of a sessile droplet on a substrate
Source: arXiv:2409.12647 ancillary file (2025-07-14)
Supplement: Supplementary file 1 [file SupplementalMaterialA.pdf]

Physical Review E, 2025

# Simulation of charged nanotubes self-assembly during evaporation of a sessile droplet on a substrate

*Konstantin S. Kolegov, Irina V. Vodolazskaya, Andrei V. Eserkepov, and Ludia T. Khusainova*

Laboratory of Mathematical Modeling, Astrakhan Tatishchev State University, Russia.

Supplementary Material A

## 1 Force of electrostatic repulsion between two charged nanotubes

Consider two charged nanotubes $A_1A_2$ and $G_1G_2$ (Fig. 1). Call them nanotubes $I$ and $II$, for short. Let the charge on each nanotube be evenly distributed along its length $l$ with the linear charge density $\sigma$.

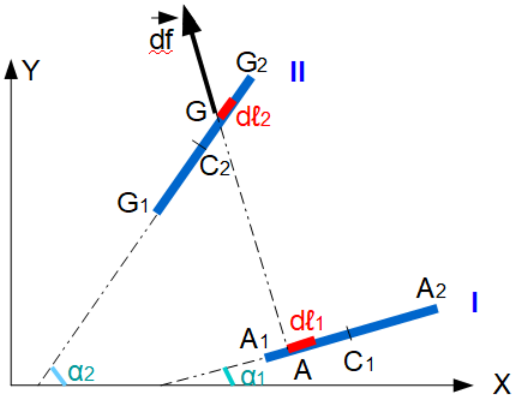


Figure 1: Graphical explanation of the derivation of the formula for the electrostatic repulsion force between two charged nanotubes.

The position of each nanotube is determined by the coordinates of its center and the angle between the particle and the $OX$ axis. For the first nanotube, there are $(x_1(C_1), y_1(C_1))$ and $\alpha_1$; for the second nanotube, we have $(x_2(C_2), y_2(C_2))$ and $\alpha_2$.

The coordinates of an arbitrary point $A$ on the first nanotube will be indexed as 1, and the coordinates of an arbitrary point $G$ on the second nanotube will be indexed as 2. The $y$-coordinate of the point on the nanotube is linearly related to its $x$-coordinate:

$$\begin{aligned} y_1 &= x_1 \cdot \tan(\alpha_1) + b_1, \\ y_2 &= x_2 \cdot \tan(\alpha_2) + b_2, \end{aligned} \tag{1}$$

where the parameters of lines, $b_1$ and $b_2$, can be determined from the coordinates of the centers of the nanotubes:

$$\begin{aligned} b_1 &= y_1(C_1) - \tan(\alpha_1) \cdot x_1(C_1), \\ b_2 &= y_2(C_2) - \tan(\alpha_2) \cdot x_2(C_2). \end{aligned} \tag{2}$$

Consider two arbitrary infinitesimal segments of the nanotube with the length $dl_1$ of the first one and the length $dl_2$ of the second one. According to Coulomb's law, the force with which the charge on segment $dl_1$ repels the charge on segment $dl_2$ is given by

$$\overrightarrow{df} = k\frac{\sigma dl_1 \cdot \sigma dl_2}{|AG|^2} \cdot \frac{\overrightarrow{AG}}{|AG|} = \\ = \frac{k\sigma^2 dl_1 \cdot dl_2}{\left(\sqrt{(x_2-x_1)^2+(y_2-y_1)^2}\right)^3} \cdot \left((x_2-x_1)\vec{n}_x + (y_2-y_1)\vec{n}_y\right), \quad (3)$$

where $k$ is the Coulomb constant, $\vec{n}_x$ and $\vec{n}_y$ are the unit vectors of the Cartesian coordinate system.

Accordingly, the force with which the nanotube $I$ repels the nanotube $II$ is given by

$$\vec{F} = \int_{A_1A_2}\int_{G_1G_2} \frac{k\sigma^2 dl_1 \cdot dl_2}{\left(\sqrt{(x_2-x_1)^2+(y_2-y_1)^2}\right)^3} \cdot \left((x_2-x_1)\vec{n}_x + (y_2-y_1)\vec{n}_y\right), \quad (4)$$

or, in terms of projections onto the coordinate axes, it is written as

$$F_x = k\sigma^2 \int_{G1_1}^{G2_2}\int_{A_1}^{A_2} \frac{x_2-x_1}{\left((x_2-x_1)^2+(y_2-y_1)^2\right)^{3/2}} \frac{dx_1dx_2}{\cos(\alpha_1)\cos(\alpha_2)}, \quad (5)$$

$$F_y = k\sigma^2 \int_{G_1}^{G_2}\int_{A_1}^{A_2} \frac{y_2-y_1}{\left((x_2-x_1)^2+(y_2-y_1)^2\right)^{3/2}} \frac{dx_1dx_2}{\cos(\alpha_1)\cos(\alpha_2)}. \quad (6)$$

After integrating, we obtain the following result for $\alpha_1 \neq \alpha_2 \neq 0 \neq \pi/2$

$$\begin{aligned} F_x &= \left.(I_2-I_1)\right|_{x_2=x_2(G_2)} - \left.(I_2-I_1)\right|_{x_2=x_2(G_1)}, \\ F_y &= \left.(I_4-I_3)\right|_{y_2=y_2(G_2)} - \left.(I_4-I_3)\right|_{y_2=y_2(G_1)}, \end{aligned} \quad (7)$$

where for $n = 1, 2$

$$I_n = \frac{k\sigma^2}{\sin(\alpha_2-\alpha_1)}\left(\sin(\alpha_2)\ln\left|\frac{x_2}{\cos(\alpha_2)} + K_n + \sqrt{\left(\frac{x_2}{\cos(\alpha_2)}+K_n\right)^2 + M_n^2}\right| + \right. \\ + \frac{\sin(\alpha_1)\cdot M_n}{\sin(\alpha_2-\alpha_1)} \cdot \left|\frac{\sin(\alpha_2-\alpha_1)}{M_n}\right| \\ \left. \cdot \ln\left|2\frac{\frac{M_n^2}{\sin^2(\alpha_2-\alpha_1)} + (K_n-N)\left(\frac{x_2}{\cos(\alpha_2)}+N\right) + \left|\frac{M_n}{\sin(\alpha_2-\alpha_1)}\right|\sqrt{\left(\frac{x_2}{\cos(\alpha_2)}+K_n\right)^2+M_n^2}}{\frac{x_2}{\cos(\alpha_2)}+N}\right|\right), \quad (8)$$

$$K_n = (b_2-b_1)\sin(\alpha_2) - x_1(A_n)\frac{\cos(\alpha_2-\alpha_1)}{\cos(\alpha_1)}, \quad (9)$$

$$M_n = (b_2-b_1)\cos(\alpha_2) + x_1(A_n)\frac{\sin(\alpha_2-\alpha_1)}{\cos(\alpha_1)}, \quad (10)$$

$$N = (b_2-b_1)\frac{\cos(\alpha_1)}{\sin(\alpha_2-\alpha_1)}, \quad (11)$$

and for $n = 3, 4$

$$I_n = -\frac{k\sigma^2}{\sin(\alpha_2-\alpha_1)}\left(\cos(\alpha_2)\ln\left|\frac{y_2}{\sin(\alpha_2)}+K_n+\sqrt{\left(\frac{y_2}{\sin(\alpha_2)}+K_n\right)^2+M_n^2}\right| - \right.$$

$$-\frac{\cos(\alpha_1)\cdot M_n}{\sin(\alpha_2-\alpha_1)}\cdot\left|\frac{\sin(\alpha_2-\alpha_1)}{M_n}\right|\cdot$$

$$\left.\cdot\ln\left|2\frac{\frac{M_n^2}{\sin^2(\alpha_2-\alpha_1)}+(K_n-H)\left(\frac{y_2}{\sin(\alpha_2)}+H\right)+\left|\frac{M_n}{\sin(\alpha_2-\alpha_1)}\right|\sqrt{\left(\frac{y_2}{\sin(\alpha_2)}+K_n\right)^2+M_n^2}}{\frac{y_2}{\cos(\alpha_2)}+H}\right|\right), \quad (12)$$

$$K_n = \left(-\frac{b_2}{\tan(\alpha_2)}+\frac{b_1}{\tan(\alpha_1)}\right)\cos(\alpha_2) - y_1(A_{n-2})\frac{\cos(\alpha_2-\alpha_1)}{\sin(\alpha_1)}, \quad (13)$$

$$M_n = \left(-\frac{b_2}{\tan(\alpha_2)}+\frac{b_1}{\tan(\alpha_1)}\right)\sin(\alpha_2) - y_1(A_{n-2})\frac{\sin(\alpha_2-\alpha_1)}{\sin(\alpha_1)}, \quad (14)$$

$$H = -\left(-\frac{b_2}{\tan(\alpha_2)}+\frac{b_1}{\tan(\alpha_1)}\right)\frac{\sin(\alpha_1)}{\sin(\alpha_2-\alpha_1)}. \quad (15)$$

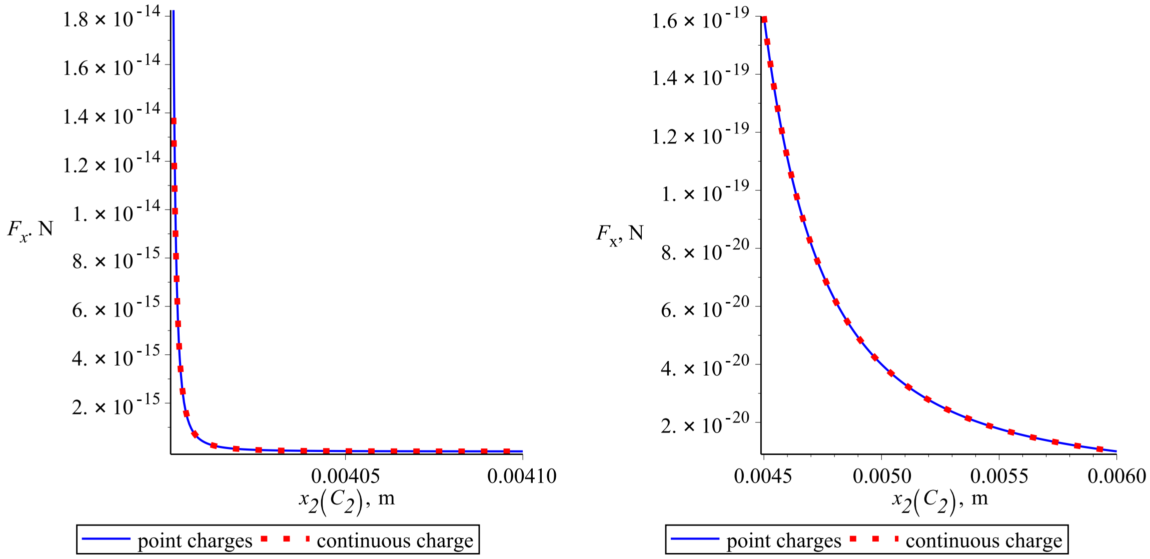


Figure 2: $x$-component of the electric force acting from the side of the nanotube $I$ on the nanotube $II$, calculated by the formula (7) (solid line) and by formula (8) of the main text of the article (dots) depending on the distance between the particles. On the left: distances of the order of the length of nanotubes. On the right: the distances are greater than the length of the nanotubes.

In the figures 2 and 3, the $x-$ and $y-$ components of the electric force acting from the nanotube $I$ on the nanotube $II$ are presented for comparison. They are calculated numerically using the formulas (7) and (8) (last one refers to the main text of the article) depending on the distance between the nanotubes (the center of mass of the first nanotube is fixed at a point $(4\cdot 10^{-3}$ m, 0), the $x$-coordinate of the center of mass of the second one changes, while its $y$-coordinate is zero; $\alpha_1 = \pi/3$, $\alpha_2 = \pi/2$). The linear charge density is $\sigma = 2q/l$, $kq^2 = 10^{-26}$ N·m$^2$.

For different tested relative positions of two nanotubes at distances between nanotubes of the order of their length, the electric force calculated in the approximation of point charges at

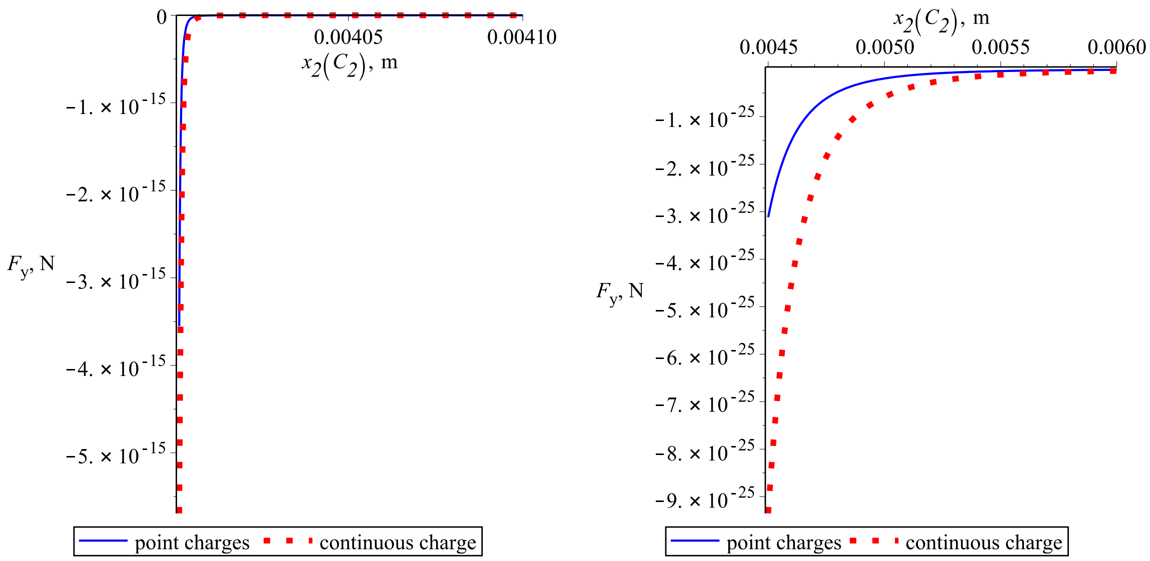


Figure 3: $y$-component of the electric force acting from the side of the nanotube $I$ on the nanotube $II$, calculated by the formula (7) (solid line) and by formula (8) of the main text of the article (dots) depending on the distance between the nanotubes. On the left: distances of the order of the length of nanotubes. On the right: the distances are greater than the length of the nanotubes.

the ends of the nanotubes exceeds in magnitude the similar force calculated for the continuous distribution of charges along the length of the nanotubes (see the left parts of Figs. 2 and 3). At distances between nanotubes greater than their length, the calculated forces coincide (see the right parts of Figs. 2 and 3).

## 2 Effect of nanotube concentration on deposit morphology

Another important issue is related to the dependence of the internal structure of the deposit on the initial concentration of the solution. To study this, calculations were performed for different numbers of particles ($N_p$ = 500, 1000, 2000, 3000, and 4000). In all cases, the results for the order parameter, $S$, are not qualitatively different (Fig. 4). Most likely, the weak side of the 2D model is manifested here. To study this dependence, it is necessary to develop a 3D model.

In Fig. 5a, a change in the local concentration (volume fraction), $\phi$, is shown for several consecutive times (advection, diffusion, and electrostatics were taken into account in the calculation). During the evaporation of the liquid and the transfer of particles, the concentration of the solution increases in the area of the droplet periphery. Despite the local increase in concentration, its value is extremely low, which confirms the validity of the assumption of constant viscosity in the model. According to the empirical formula [1]

$$\eta = 0.9775\eta_0 \left(1 + \frac{T - 273}{70}\right)^{0.26087} (1+\phi)^{8.13792},$$

the viscosity value of the solution, $\eta$, varies within 8.5% in the range of values of $\phi$ from $10^{-5}$ to $10^{-2}$. If a higher concentration is achieved, it obviously occurs at the end of the evaporation process, outside the fixing radius. In the future, when dealing with concentrated solutions and multilayer deposits, it is important to take into account the viscosity dependence on concentration when calculating hydrodynamics.

The local particle velocity, $v_p$, for different time points is shown in Fig. 5b. These numerical results are qualitatively agree with the results of calculations of the solution flow velocity based

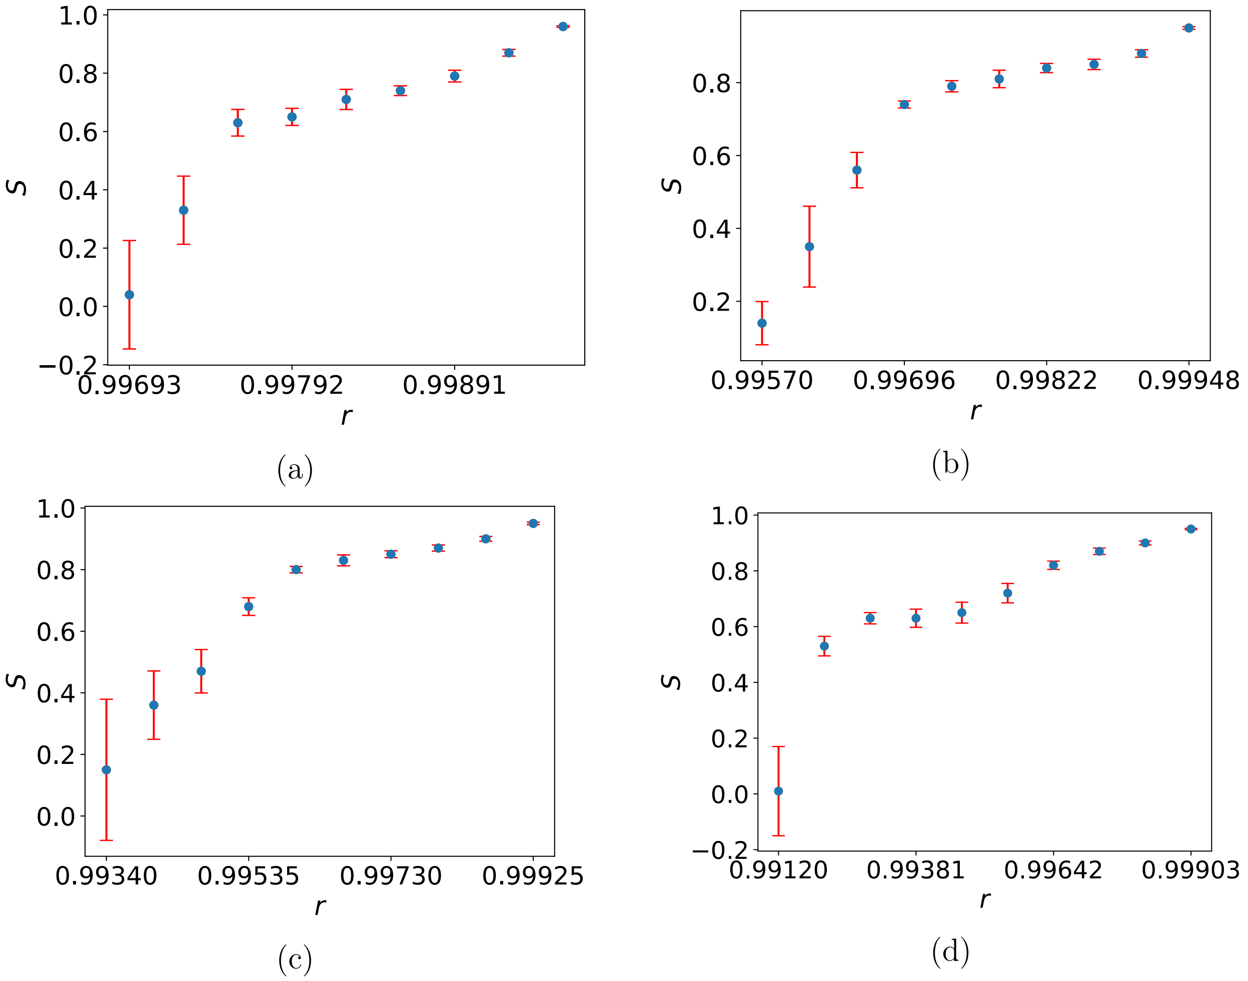


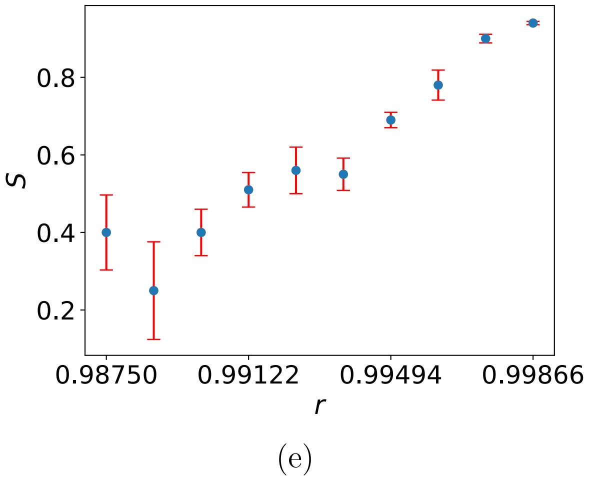


Figure 4: Calculation results of the order parameter, $S$, for different values of $N_p$: (a) 500, (b) 1000, (c) 2000, (d) 3000, and (e) 4000 (taking into account advection, diffusion and electrostatic interaction at $kq^2 = 10^{-26}$ m$^2$N and $t_{\max} = 200$ s).

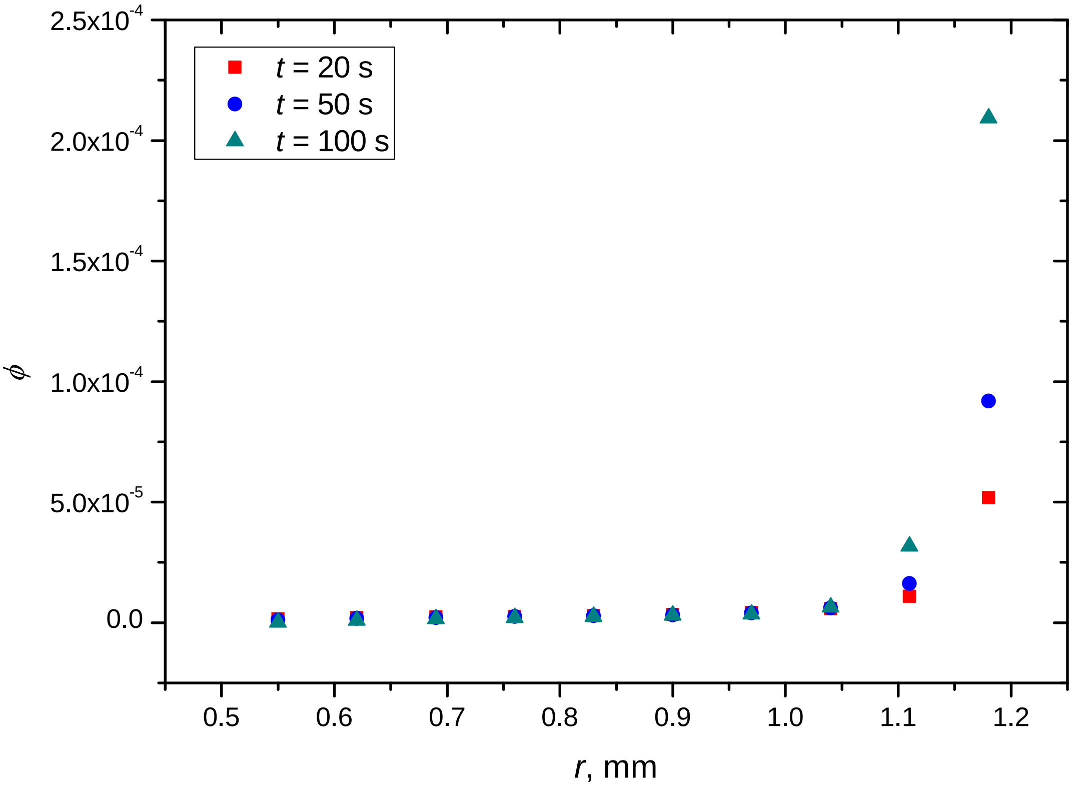


(a)

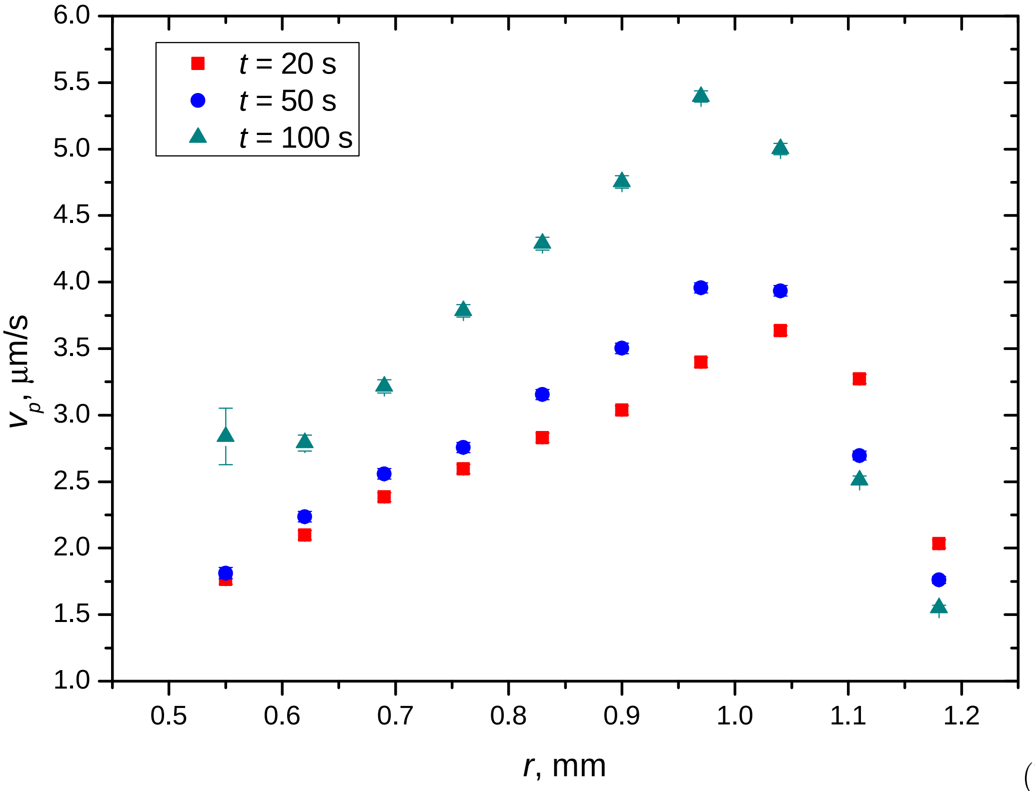


(b)

Figure 5: Dependence of (a) the concentration and (b) the velocity of particles on the radial coordinate for several time points ($N_p = 3000$, $t_{\max} = 200$ s, $kq^2 = 10^{-26}$ m$^2$N).

on the continual model [2] (see Fig. 3c [2]). Note that the value of $v_p$ increases in almost the entire region (Fig. 5b). Only near the contact line does particle velocity decrease over time due to an increase in their concentration. In our model, this is explained by the fact that as the concentration increases, the particles in this region interfere more with each other through

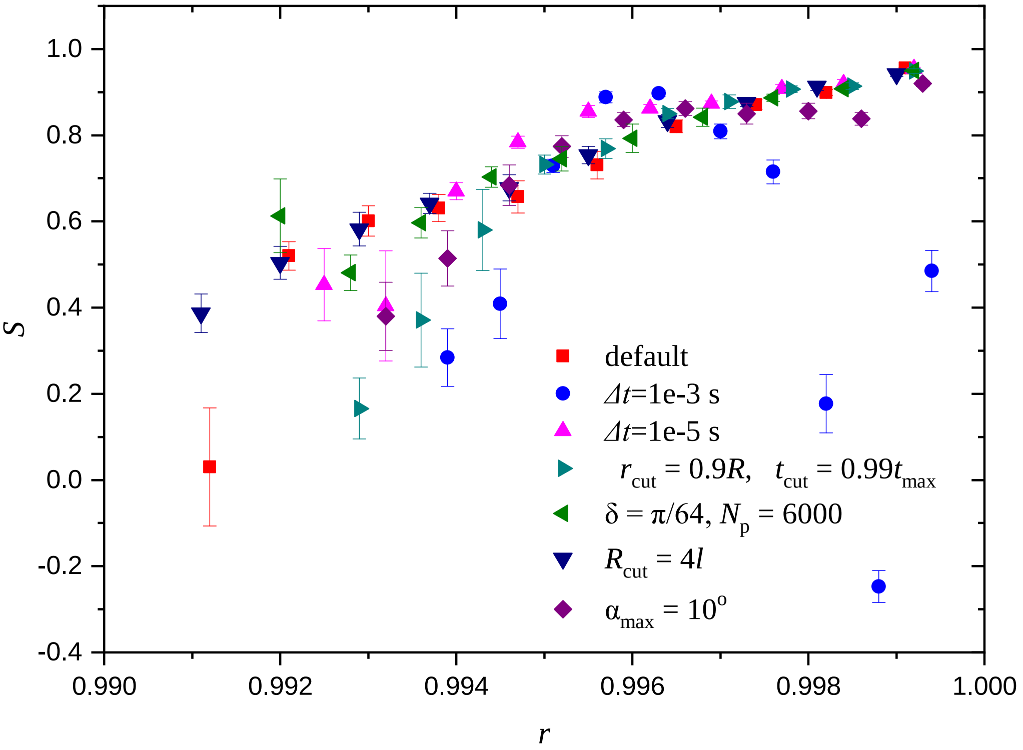


Figure 6: Dependence of the order parameter on the coordinate for the final nanotube structure (default parameter values: $N_p = 3000$, $t_{\max} = 200$ s, $kq^2 = 10^{-26}$ m$^2$N, $\Delta t = 10^{-4}$ s, $R_{\text{cut}} = 3l$, $r_{\text{cut}} = 0.85R$, $t_{\text{cut}} = 0.98t_{\max}$, $\delta = \pi/128$, and $\alpha_{\max} = 1°$).

mechanical collisions and electrostatic interactions. In the model [2], a slowdown in solution flow velocity over time near the contact line is associated with an increase in viscosity due to an increase in local concentration leading to a "sol–gel" phase transition. In Ref. [2] a concentrated solution is considered ($\phi_0 = 0.15$). It is worth noting that the continual model [2] does not describe the mechanical and electrostatic interaction of particles. It does not take into account the shape of particles or predict the morphology of deposits. Only its geometry is predicted.

# 3 Analysis of the parameters of the numerical method

In Fig. 6, the result of the calculation of the order parameter, $S$, is presented, taking into account advection, diffusion, and electrostatics. The caption to this figure lists default parameter values. To test the effect of parameters related to numerical methods on the results, both their default values and other values were used. We are talking about such parameters as the time step $\Delta t$, the cutting radius $R_{\text{cut}}$ to account for the electrostatic interaction of particles, the parameters for solving the problem of singular flow velocity $r_{\text{cut}}$ and $t_{\text{cut}}$, the sector angle $\delta$, and the maximum rotation angle of the nanotube $\alpha_{\max}$.

With a relatively large time step ($\Delta t = 10^{-3}$ s), the calculation result does not agree with the experiment (see Fig. 3 in Ref. [3]). In contrast, at small step values ($\Delta t = 10^{-4}$ s and $10^{-5}$ s), a transition from disorder to alignment is observed as the coordinate $r$ increases. The calculation results for $\Delta t = 10^{-4}$ s and $10^{-5}$ s agree well with each other (Fig. 6), but the calculation takes an order of magnitude less time at $\Delta t = 10^{-4}$ s.

Increasing the cutting radius $R_{\text{cut}}$ from $3l$ to $4l$ has no qualitative effect on the result. The quantitative difference is noticeable only at the leftmost point (Fig. 6). This is because in that subdomain, there are particles that are furthest away from densely packed nanotubes on the periphery. The width of the deposit is approximately $w = 7.5l$. At the same time, increasing

$R_{\text{cut}}$ makes the problem computationally expensive. The force of interaction between particles is inversely proportional to the square of the distance between them. So, the long-range nature of the interaction can be ignored. Here, we do not claim to quantitative results, but rather study the process at a qualitative level. Of course, if it is necessary to obtain more accurate data, one should try to increase $R_{\text{cut}}$ in order to achieve optimal accuracy of the result, taking into account the time cost of calculations.

To study the effect of the size of the calculated area with periodic boundary conditions on the simulation results, additional calculations were performed using a doubled sector angle ($\delta = \pi/64$). At the same time, the number of particles was increased proportionally ($N_p = 6000$) to maintain the same particle concentration. In Fig. 6, the calculation results for $\delta = \pi/64$ and $\delta = \pi/128$ agree well with each other.

Let us pay attention to the limit of the nanotube rotation angle $\alpha_{\max}$ in one time step. If we enlarge $\alpha_{\max}$ from 1 to 10°, one observes that the same trend of rising the value of $S$ persists as the coordinate $r$ increases. However, there is a noticeable quantitative difference at the point $r \approx 0.993$, where $S \approx 0.4$ for $\alpha_{\max} = 10°$ and $S \approx 0.6$ for $\alpha_{\max} = 1°$. This is most likely due to the fact that, for $\alpha_{\max} = 10°$, the width of the annular deposit $w$ is about 22.2% less (Fig. 6). The reason for this may be a denser packing of particles. In our model, the artificial limitation of the rotation angle is a compulsory measure. It is most likely that viscous friction, which damps the rotational impulse, needs to be simulated more accurately. In the future, in order to move from conceptual modeling to detailed one, it will be necessary to pay attention to this issue, among other things.

One should also understand how the choice of the values of parameters $r_{\text{cut}}$ and $t_{\text{cut}}$ affects the results of calculations. By default, the values of parameters $r_{\text{cut}} = 0.85R$ and $t_{\text{cut}} = 0.98t_{\max}$ are used. For comparison, we increase their values, for example, $r_{\text{cut}} = 0.9R$ and $t_{\text{cut}} = 0.99t_{\max}$. In this case, we get the maximum value of the flow velocity about $v_{\max} = 239$ $\mu$m/s, which is significantly higher than $v_{\max} \approx 60$ $\mu$m/s [4]. The value of $v_{\max} = 239$ $\mu$m/s is obtained if we take into account the parameters ($R \approx 0.45$ mm, $t_{\max} \approx 110$ s) from the experiment [4]. For our case ($R \approx 1.25$ mm, $t_{\max} \approx 200$ s), the estimated velocity will be even higher. Note that for different values of $r_{\text{cut}}$ and $t_{\text{cut}}$, there are no noticeable differences in the qualitative behavior of $S$ (Fig. 6). The quantitative differences are related to the fact that for $r_{\text{cut}} = 0.9R$ and $t_{\text{cut}} = 0.99t_{\max}$, the width of the annular deposit, $w$, is approximately 21% less. The reason for this may be a higher (overestimated) flow velocity at the periphery, which leads to a strong pressing of the nanotubes to the edge (denser packing).

# References


[1] Le Ba T, Alkurdi A Q, Lukács I E, Molnár J, Wongwises S, Gróf G and Szilágyi I M 2020 *Nanomaterials* **10** 1834 ISSN 2079-4991

[2] Park Y, Park Y, Lee J and Lee C 2019 *Journal of Applied Physics* **125** 065304

[3] Zhao Y, Cavallaro G and Lvov Y 2015 *Journal of Colloid and Interface Science* **440** 68–77

[4] Hamamoto Y, Christy J R E and Sefiane K 2011 *Physical Review E* **83** 051602
